# Supplementary material for: First-principles Spin and Optical Properties of Vacancy Clusters in Lithium Fluoride
Source: arXiv:2412.21060 ancillary file (2024-12-31)
Supplement: Supplementary file 1 [file Supplementary_Material.pdf]

Supplementary Material: First-principles Spin and Optical Properties of Vacancy Clusters in Lithium Fluoride

Mariano Guerrero Perez[1], Keegan Walkup[1], Jordan Chapman[2], Pranshu Bhaumik[4], Giti A. Khodaparast[1], Brenden A. Magill[1], Patrick Huber[1], and Vsevolod Ivanov[1,2,3]

[1]Department of Physics, Virginia Tech, Blacksburg, Virginia 24061, USA
[2]Virginia Tech National Security Institute, Blacksburg, Virginia 24060, USA
[3]Virginia Tech Center for Quantum Information Science and Engineering, Blacksburg, Virginia 24061, USA
[4]College of William and Mary, Williamsburg, VA 23187, USA

## Supplementary Note 1: Description of computed spin and optical properties.

**Absorption/Emission Energies**. Due to the strong electron-phonon coupling of some defects in lithium fluoride, the standard method of computing the zero-phonon line energy ($\Delta E_{\text{ZPL}}$) of optical transitions in color center defects is inadequate. Normally to compute $\Delta E_{\text{ZPL}}$ by the $\Delta$-SCF method [S1], the free energy of the ground state, $E_{\text{GS}}$ is obtained by minimizing the forces to find the relaxed atomic positions in the ground state, $q_{\text{GS}}$. This is subtracted from the free energy with the occupations constrained to the excited state $E_{\text{EX}}$ and forces minimized again to obtain the relaxed excited state atomic positions, $q_{\text{EX}}$, to obtain

$$\Delta E_{\text{ZPL}} = E_{\text{EX}}(q_{\text{EX}}) - E_{\text{GS}}(q_{\text{GS}})$$

In the presence of strong electron-phonon coupling, ground ($q_{\text{GS}}$) and excited state ($q_{\text{EX}}$) configurations may differ significantly, with optically active electronic transitions taking place quickly enough that the atomic configuration of the defect doesn't change. In between these absorption and emission processes, the atomic configuration undergoes non-radiative relaxation. The energies of the absorption ($\Delta E_{\text{ABS}}$) and emission ($\Delta E_{\text{EMIT}}$)processes can therefore be approximated as

$$\Delta E_{\text{ABS}} = E_{\text{EX}}(q_{\text{GS}}) - E_{\text{GS}}(q_{\text{GS}})$$
$$\Delta E_{\text{EMIT}} = E_{\text{EX}}(q_{\text{EX}}) - E_{\text{GS}}(q_{\text{EX}})$$

**Transition Dipole Moment**. The transition dipole moment is given by

$$\boldsymbol{\mu} = \frac{i\hbar}{m_e}\frac{\langle\psi_f|\boldsymbol{p}|\psi_i\rangle}{E_f - E_i}$$

where $\psi_i/\psi_f$ are the initial/final states with energies $E_i/E_f$, $\boldsymbol{p}$ is the momentum operator, and $m_e$ is the electron mass.
**Radiative Lifetime**. The radiative lifetime $\tau$ is given by Wigner-Weisskopf fluorescence theory [S1, S2] as

$$\tau = \frac{3\epsilon_0 hc^3}{n_r(2\pi)^3\nu^3|\boldsymbol{\mu}|^2}$$

where $\epsilon_0$ is the vacuum permittivity, $h$ is Planck's constant, $c$ is the speed of light, $n_r = 1.39$ is the refractive index of LiF [S3], $\nu = \Delta E/h$ is the frequency of the transition, and $\boldsymbol{\mu}$ is the transition dipole moment.
**Zero Field Splitting**. The spin-spin interaction can be written [S4]:

$$H_{ss} = \boldsymbol{SDS} = -\frac{\mu_0}{4\pi}\frac{g^2\mu_B^2}{r^3}\left(\frac{3}{4}(\boldsymbol{s}_1\cdot\hat{\boldsymbol{r}})(\boldsymbol{s}_2\cdot\hat{\boldsymbol{r}}) - \boldsymbol{s}_1\cdot\boldsymbol{s}_2\right), \quad (1)$$

where $\mu_0$ is the magnetic permeability, $g$ is the Landé g-factor, $\mu_B$ is the Bohr magneton, $\boldsymbol{S} = \boldsymbol{s}_1 + \boldsymbol{s}_2$ is the total spin with $\boldsymbol{s}_i = \frac{1}{2}[\sigma_x, \sigma_y, \sigma_z]$ being the spin operator for particle $i$, and $\sigma_x, \sigma_y, \sigma_z$ are the Pauli matrices. $\boldsymbol{D}$ is the traceless dipole-dipole interaction tensor, that is $D_{xx} + D_{yy} + D_{zz} = 0$, and when computed in VASP, the tensor elements are automatically ordered by magnitude $D_{zz} > D_{yy} > D_{xx}$. For a triple state, the spin-spin interaction results in a $3\Delta$ gap between the $m_s = 0$ and $m_s = \pm 1$ where

$$3\Delta = -\frac{3}{4}D_{zz} = 3\frac{\mu_0}{4\pi}g^2\mu_B^2\left\langle\psi\left|\frac{1-3\hat{z}^2}{4r^3}\right|\psi\right\rangle. \quad (2)$$

## Supplementary Note 2: Electronic structures and properties of LiF color center triplet states.

In this section we provide information on the triplet states of the $F_2^0$-center, $F_3^-$-center, and $F_3^+$-center, including their electronic structures, energy relative to the singlet ground state, and zero-field splitting tensor elements.

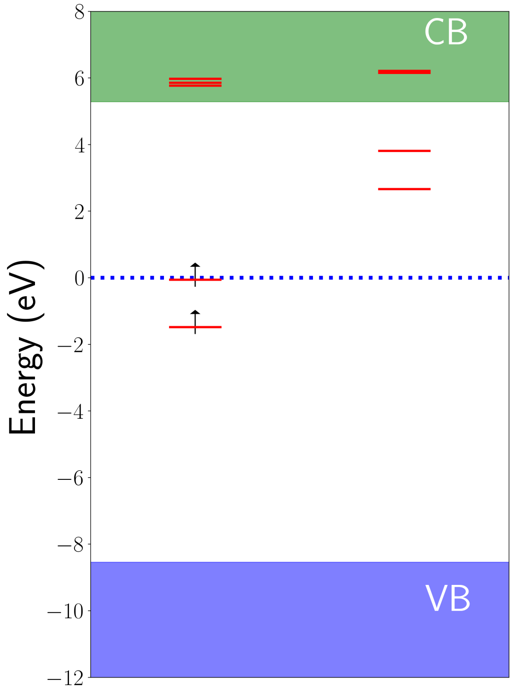


$$E_{\mathrm{GS}}^{\boldsymbol{S}=0} - E_{\mathrm{GS}}^{\boldsymbol{S}=1} = -290 \text{ meV}$$

| | eigenvector |
|---|---|
| $D_{xx} = 766$ MHz | $(0.000, 0.707, 0.707)$ |
| $D_{yy} = 838$ MHz | $(1.000, 0.000, 0.000)$ |
| $D_{zz} = -1603$ MHz | $(0.000, 0.707, -0.707)$ |

Figure S1: Electronic structure of the $F_2^0$-center triplet state.

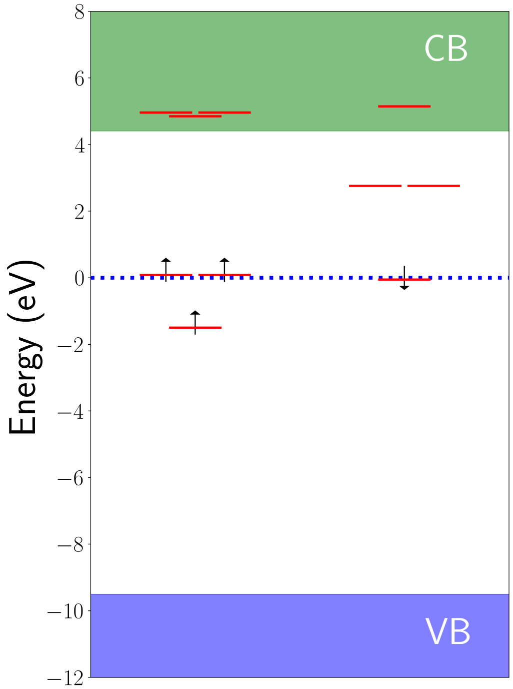


$$E_{\mathrm{GS}}^{\boldsymbol{S}=0} - E_{\mathrm{GS}}^{\boldsymbol{S}=1} = 266 \text{ meV}$$

| | eigenvector |
|---|---|
| $D_{xx} = -2199$ MHz | $(0.268, -0.802, 0.534)$ |
| $D_{yy} = -2199$ MHz | $(-0.771, 0.153, 0.618)$ |
| $D_{zz} = 4399$ MHz | $(-0.577, -0.577, -0.577)$ |

Figure S2: Electronic structure of the $F_3^-$-center triplet state.

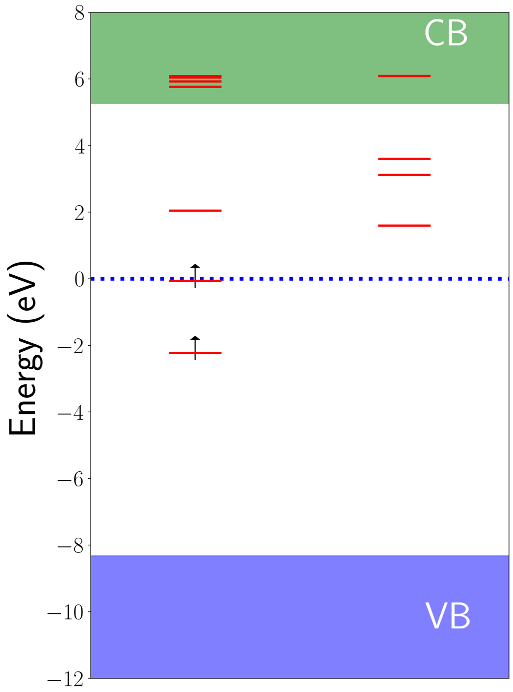


$$E_{\mathrm{GS}}^{\boldsymbol{S}=0} - E_{\mathrm{GS}}^{\boldsymbol{S}=1} = -884 \text{ meV}$$

| | eigenvector |
|---|---|
| $D_{xx} = -103$ MHz | $(0.493, 0.717, 0.493)$ |
| $D_{yy} = -1436$ MHz | $(-0.507, 0.697, -0.507)$ |
| $D_{zz} = 1539$ MHz | $(-0.707, 0.000, 0.707)$ |

Figure S3: Electronic structure of the $F_3^+$-center triplet state.

## References


[S1] Adam Gali, Erik Janzén, Péter Deák, Georg Kresse, and Efthimios Kaxiras. Theory of spin-conserving excitation of the $n - V^-$ center in diamond. *Phys. Rev. Lett.*, 103:186404, Oct 2009.

[S2] Audrius Alkauskas, Cyrus E. Dreyer, John L. Lyons, and Chris G. Van de Walle. Role of excited states in shockley-read-hall recombination in wide-band-gap semiconductors. *Phys. Rev. B*, 93:201304, May 2016.

[S3] H. H. Li. Refractive index of alkali halides and its wavelength and temperature derivatives. *Journal of Physical and Chemical Reference Data*, 5(2):329–528, 04 1976.

[S4] J R Maze, A Gali, E Togan, Y Chu, A Trifonov, E Kaxiras, and M D Lukin. Properties of nitrogen-vacancy centers in diamond: the group theoretic approach. *New Journal of Physics*, 13(2):025025, feb 2011.
